# Supplementary material for: EPMF: Efficient Perception-aware Multi-sensor Fusion for 3D Semantic Segmentation
Source: arXiv:2106.15277 source file (2026-07-04)
Supplement: Supplementary file 1 [file 03293-supp.pdf]

# Supplementary Material for “Perception-Aware Multi-Sensor Fusion for 3D LiDAR Semantic Segmentation”

Zhuangwei Zhuang<sup>1,2</sup> Rong Li<sup>1,2</sup> Kui Jia<sup>1</sup> Qicheng Wang<sup>3</sup> Yuanqing Li<sup>2,1†</sup> Mingkui Tan<sup>1,2†</sup>

<sup>1</sup>South China University of Technology <sup>2</sup>Pazhou Lab <sup>3</sup>Shenzhen Youjia Innov Tech Co., Ltd

{z.zhuangwei, selirong}@mail.scut.edu.cn, wangqicheng@minieye.cc

{auyqli, kuijia, mingkuitan}@scut.edu.cn

We organize our supplementary material as follows.

- In Section 1, we introduce the details of the two additional losses, namely, multi-class focal loss and Lovász-softmax loss, in the objective of Perception-aware Multi-sensor Fusion (PMF).
- In Section 2, we give more implementation details of PMF.
- In Section 3, we investigate the effect of the proposed residual-based fusion module.
- In Section 4, we study the effect of hyperparameters  $\tau, \gamma, \lambda$ .
- In Section 5, we provide more visualization results of PMF on SemanticKITTI validation set.
- In Section 6, we show more visualization results of PMF on nuScenes validation set.
- In Section 7, we give more visualization results of PMF on the adversarial samples.

## 1. Details of the Loss Functions

For convenience, we show the architecture of PMF in Figure 1. In Section 3.3 of the main paper, we have introduced the objective of PMF. Specifically, we propose the perception-aware losses to measure the vast perceptual difference between the data from RGB camera and LiDAR. Following [2, 6], we use the multi-class focal loss [4] to address the class imbalance issue and Lovász-softmax loss [1] to measure the scale variance in semantic segmentation, respectively. Therefore, the objective  $\tilde{\mathcal{L}}$  w.r.t. the LiDAR stream in two-stream network (TSNet) is defined as

$$\tilde{\mathcal{L}} = \tilde{\mathcal{L}}_{foc} + \lambda \tilde{\mathcal{L}}_{lov} + \gamma \tilde{\mathcal{L}}_{per},$$

where  $\tilde{\mathcal{L}}_{foc}, \tilde{\mathcal{L}}_{lov}, \tilde{\mathcal{L}}_{per}$  indicate the multi-class focal loss, Lovász-softmax loss and perception-aware loss w.r.t. the LiDAR stream, respectively. Here,  $\gamma$  and  $\lambda$  are hyper-parameters. The objective  $\mathcal{L}$  w.r.t. the camera stream in TSNet is defined as

$$\mathcal{L} = \mathcal{L}_{foc} + \lambda \mathcal{L}_{lov} + \gamma \mathcal{L}_{per},$$

where  $\mathcal{L}_{foc}, \mathcal{L}_{lov}, \mathcal{L}_{per}$  indicate the multi-class focal loss, Lovász-softmax loss and perception-aware loss w.r.t. the camera stream, respectively.

In this section, we give the details of the multi-class focal loss [4] and Lovász-softmax loss [1] in the objective of PMF. Let  $\{\mathbf{P}, \mathbf{X}, \mathbf{y}\}$  be one of the training samples from a given data set, where  $\mathbf{P} \in \mathbb{R}^{4 \times N}$  indicates a point cloud,  $N$  denotes the number of points. Each point  $\mathbf{P}_i = (x, y, z, r)^\top$  consists of 3D coordinates  $(x, y, z)$  and an reflectance value  $(r)$ .  $\mathbf{y} \in \mathbb{R}^N$  denotes the semantic labels for point cloud  $\mathbf{P}$ . Let  $\mathbf{Y} \in \mathbb{R}^{H \times W}$  be the projected labels in the camera coordinates.  $H$  and  $W$  indicate the height and width, respectively. For each point  $\mathbf{P}_i$ , we project the 3D coordinates  $(x, y, z)$  to the pixel  $(h, w)$  in the camera coordinate system by using perspective projection. Then, we initialize all pixels in  $\mathbf{Y}$  by 0 and compute the projected labels in  $\mathbf{Y}$  by

$$\mathbf{Y}_{h,w} := \mathbf{y}_i.$$

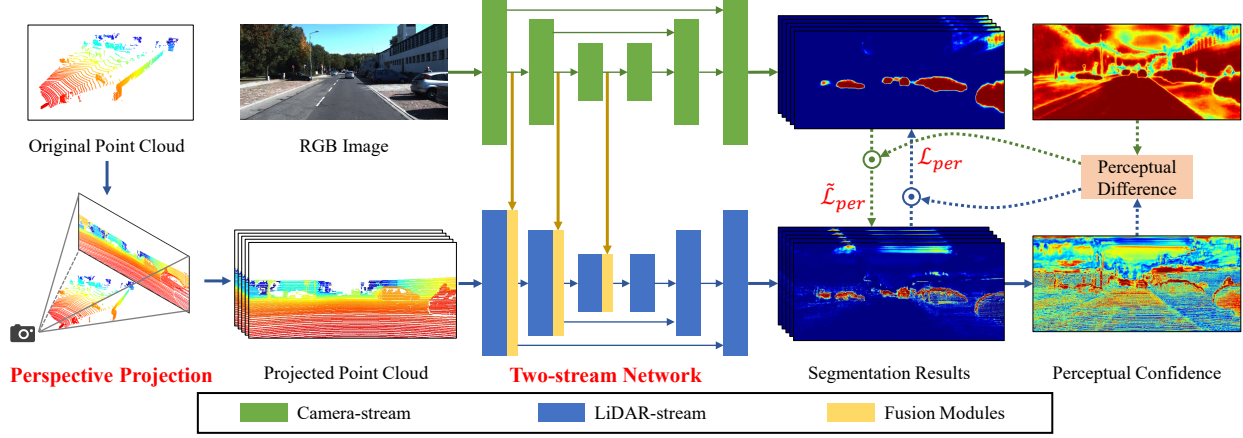

Figure I. Illustration of perception-aware multi-sensor fusion (PMF). PMF consists of three components: (1) perspective projection; (2) a two-stream network (TSNet) with feature fusion modules; and (3) perception-aware losses  $\mathcal{L}_{per}$ ,  $\tilde{\mathcal{L}}_{per}$  w.r.t. the camera stream and the LiDAR stream, respectively. We first project the point clouds to camera coordinate with perspective projection and learn the features from both RGB images and point clouds using TSNet. Then, the image features are fused into the LiDAR stream network by fusion modules. Last, we use perception-aware losses to measure the perceptual difference between the two modalities.

**Multi-class focal loss.** Let  $FL(p) = -(1 - p)^2 \log(p)$  be the focal-loss function.  $\tilde{\mathbf{O}} \in \mathbb{R}^{S \times H \times W}$  indicates the output probabilities of the LiDAR stream, where  $S$  denotes the number of classes. The multi-class focal loss w.r.t. the LiDAR stream is defined as

$$\tilde{\mathcal{L}}_{foc} = \frac{1}{K} \sum_{s=1}^S \sum_{h=1}^H \sum_{w=1}^W \mathbb{1}\{\mathbf{Y}_{h,w} = s\} FL(\tilde{\mathbf{O}}_{s,h,w}),$$

where  $K = \sum_{s=1}^S \sum_{h=1}^H \sum_{w=1}^W \mathbb{1}\{\mathbf{Y}_{h,w} = s\}$  indicates the number of available labels.  $\mathbb{1}\{\cdot\}$  indicates the indicator function. Let  $\mathbf{O} \in \mathbb{R}^{S \times H \times W}$  denotes the output probabilities of the camera stream. Then, the multi-class focal loss w.r.t. the camera stream is

$$\mathcal{L}_{foc} = \frac{1}{K} \sum_{s=1}^S \sum_{h=1}^H \sum_{w=1}^W \mathbb{1}\{\mathbf{Y}_{h,w} = s\} FL(\mathbf{O}_{s,h,w}),$$

**Lovász-softmax loss.** The Lovász-softmax loss w.r.t. the LiDAR stream is defined as

$$\tilde{\mathcal{L}}_{lov} = \frac{1}{S} \sum_{s=1}^S \overline{\Delta_{J_s}}(\tilde{\mathbf{m}}(s)),$$

where

$$\tilde{\mathbf{m}}_i(s) = \begin{cases} 1 - \tilde{\mathbf{O}}_{s,h,w} & \text{if } s = \mathbf{Y}_{h,w}, \\ \tilde{\mathbf{O}}_{s,h,w} & \text{otherwise.} \end{cases}$$

$\overline{\Delta_{J_s}}$  indicates the Lovász extension of the Jaccard index for class  $s$ . Here,  $(h, w)$  is obtained from the 3D coordinates  $(x, y, z)$  of  $\mathbf{P}_i$  by using perspective projection.  $\tilde{\mathbf{m}}(s) \in [0, 1]^N$  indicates the vector of errors. The Lovász-softmax loss w.r.t. the camera stream is defined as

$$\mathcal{L}_{lov} = \frac{1}{S} \sum_{s=1}^S \overline{\Delta_{J_s}}(\mathbf{m}(s)),$$

where

$$\mathbf{m}_i(s) = \begin{cases} 1 - \mathbf{O}_{s,h,w} & \text{if } s = \mathbf{Y}_{h,w}, \\ \mathbf{O}_{s,h,w} & \text{otherwise.} \end{cases}$$

## 2. More Implementation Details of PMF

In this section, we give more implementation details of PMF. We first discuss the number of fusion modules in the two-stream network (See Figure I) and then introduce the method to obtain the sparse predictions from the dense ones.

**Number of fusion modules.** In Figure I, we insert  $L$  fusion modules into the LiDAR stream to fuse the features from the camera. Note that one can add the fusion modules after each layer in the network. However, this can be computationally expensive yet unnecessary. Inspired by [3, 5], we only insert four fusion modules into the LiDAR stream to fuse the multi-scale features from the camera stream. Specifically, we fuse the camera features from the 7-th, 15-th, 27-th, 33-th convolutional layers of ResNet-34 into the LiDAR features from the 14-th, 19-th, 24-th, 29-th convolutional layers of SalsaNext, respectively.

**Method to obtain the sparse predictions.** With the proposed perception-aware losses, PMF generates dense segmentation results with information from RGB images and point clouds. We then obtain the sparse prediction from the dense results. Let  $\tilde{\mathbf{O}} \in \mathbb{R}^{S \times H \times W}$  be the output probabilities of the LiDAR stream.  $S$  indicates the number of classes.  $H$  and  $W$  indicate the height and width of the predictions, respectively. Let  $\hat{\mathbf{Y}} \in \mathbb{R}^{H \times W}$  be the dense predictions from the LiDAR stream. Then, the dense predictions is computed by

$$\hat{\mathbf{Y}}_{h,w} = \arg \max_s \tilde{\mathbf{O}}_{s,h,w}.$$

Let  $\hat{\mathbf{y}} \in \mathbb{R}^N$  be the sparse predictions of point cloud  $\mathbf{P}$ . As shown in Figure II, for each point  $\mathbf{P}_i$ , we first project the 3D coordinates  $(x, y, z)$  to the camera coordinate system by using perspective projection and compute the corresponding pixel  $(h, w)$  in the projected image. Then the semantic prediction  $\hat{\mathbf{y}}_i$  w.r.t. the point  $\mathbf{P}_i$  is computed by

$$\hat{\mathbf{y}}_i := \hat{\mathbf{Y}}_{h,w}.$$

Note that for the point cloud with multi-camera views, *e.g.*, nuScenes, there are overlaps between different camera views. To address this issue, we first run forward propagation for each camera view and merge the results by assigning the predictions with the highest confidence scores to the points in the overlaps of different views.

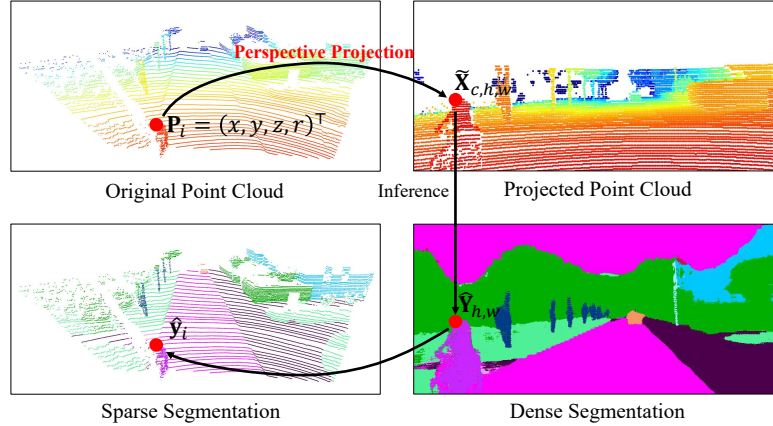

Figure II. Illustration of the pipeline to obtain the sparse segmentation from the dense prediction results.  $\tilde{\mathbf{X}}$  indicates the projected point cloud.  $\hat{\mathbf{Y}}$  and  $\hat{\mathbf{y}}$  indicate the dense predictions and sparse predictions, respectively. For each point  $\mathbf{P}_i$ , we first compute the corresponding pixel  $(h, w)$  in the camera coordinate system by perspective projection. Second, we get the dense segmentation  $\hat{\mathbf{Y}}$  from the prediction results of PMF. Last, we obtain the corresponding sparse prediction  $\hat{\mathbf{y}}_i$  w.r.t. the point  $\mathbf{P}_i$  from the dense segmentation  $\hat{\mathbf{Y}}_{h,w}$ .

### 3. Effect of Residual-based Fusion Module

In Section 3.2 of the main paper, we have proposed the residual-based fusion (RF) modules to fuse the features from RGB images into the LiDAR stream. To investigate the effect of components in RF modules, we replace the fusion modules in PMF with two variants of RF modules (see Figure III) and evaluate the performance on SemanticKITTI. From Table A, the residual connection improves the performance by 1.2% in mIoU. Besides, the attention module yields an improvement of 0.8% in mIoU. These results demonstrate the effectiveness of each component in the proposed residual-based fusion module.

To further study the effect of the proposed residual-based fusion modules, we visualize the features of the first fusion module in PMF. From Figure IV, features from RGB images provide more appearance information (*e.g.*, texture) than those from point clouds. With the proposed fusion module, PMF is able to fuse both information from RGB camera and LiDAR. Besides, the noises from RGB images (*e.g.*, the shadows of trees) are also reduced during feature fusion.

Table A. Comparisons of different fusion modules. The **bold** number indicates the best result.

| Fusion Module | Module A | Module B | Residual-based Fusion (Ours) |
|---------------|----------|----------|------------------------------|
| mIoU (%)      | 61.9     | 63.1     | <b>63.9</b>                  |

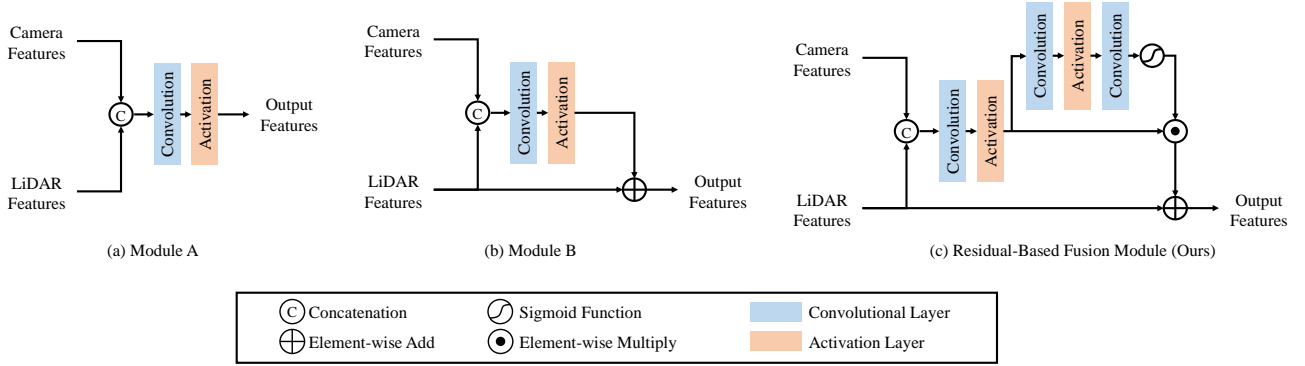

Figure III. Illustration of different fusion modules. (a) indicates the naive concatenation fusion, (b) indicates the naive concatenation with residual connection, (c) indicates our residual-based fusion module.

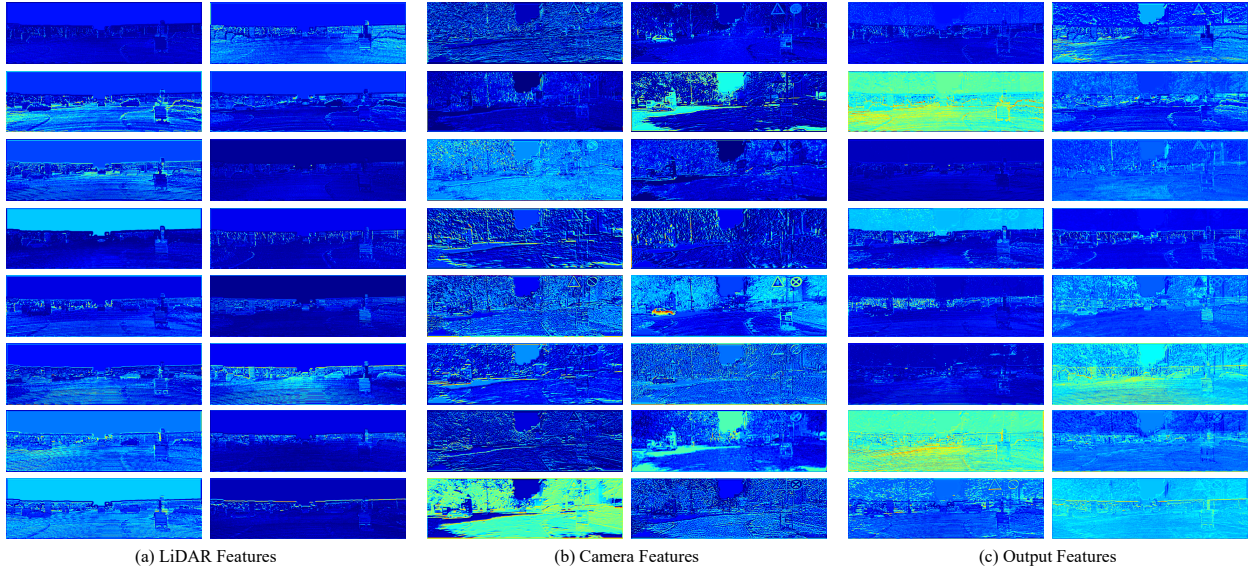

Figure IV. Visualization of features of the first residual-based fusion module in PMF. For clarity, we only visualize the first 16 feature maps of the LiDAR features, camera features, and output features.

#### 4. Effect of hyperparameters $\tau, \gamma, \lambda$

To investigate the effect of  $\tau$ , we first set  $\lambda$  and  $\gamma$  to 1 and train PMF with  $\tau \in \{0.1, 0.3, 0.5, 0.7, 0.9\}$  on SemanticKITTI. From Table B, the model with  $\tau = 0.7$  achieves the best performance on the benchmark data set. We then set  $\tau = 0.7$  and  $\lambda = 1$  to train models with  $\gamma \in \{0.0, 0.5, 1.0, 5.0, 10.0\}$ . From Table C, PMF achieves the best performance with  $\gamma = 0.5$ . Last, we set  $\tau$  to 0.7 and  $\gamma$  to 0.5 to train models with  $\lambda \in \{0.0, 0.5, 1.0, 1.5, 2.0\}$ . From Table D, the model with  $\lambda = 1.0$  achieves the best result on the data set. Therefore, in our experiments, we set  $\tau, \gamma, \lambda$  to 0.7, 0.5, and 1.0.

Table B. Effect of  $\tau$ . We highlight the best result in bold.

| $\tau$   | 0.1  | 0.3  | 0.5  | 0.7         | 0.9  |
|----------|------|------|------|-------------|------|
| mIoU (%) | 63.2 | 63.2 | 63.2 | <b>63.6</b> | 63.5 |

Table C. Effect of  $\gamma$ . We highlight the best result in bold.

| $\gamma$ | 0.0  | 0.5         | 1.0  | 5.0  | 10.0 |
|----------|------|-------------|------|------|------|
| mIoU (%) | 61.7 | <b>63.9</b> | 63.6 | 63.7 | 63.6 |

Table D. Effect of  $\lambda$ . We highlight the best result in bold.

| $\lambda$ | 0.0  | 0.5  | 1.0         | 1.5  | 2.0  |
|-----------|------|------|-------------|------|------|
| mIoU (%)  | 61.6 | 63.0 | <b>63.9</b> | 62.6 | 62.6 |

## 5. More Visualization Results on SemanticKITTI

In Section 4.4 of the main paper, we have provided the qualitative results on SemanticKITTI. In this section, we give more visualization results on SemanticKITTI in Figure V. From the results, our PMF is robust to different lighting conditions in RGB images, such as the shadows of trees and exposure on the surface of buildings.

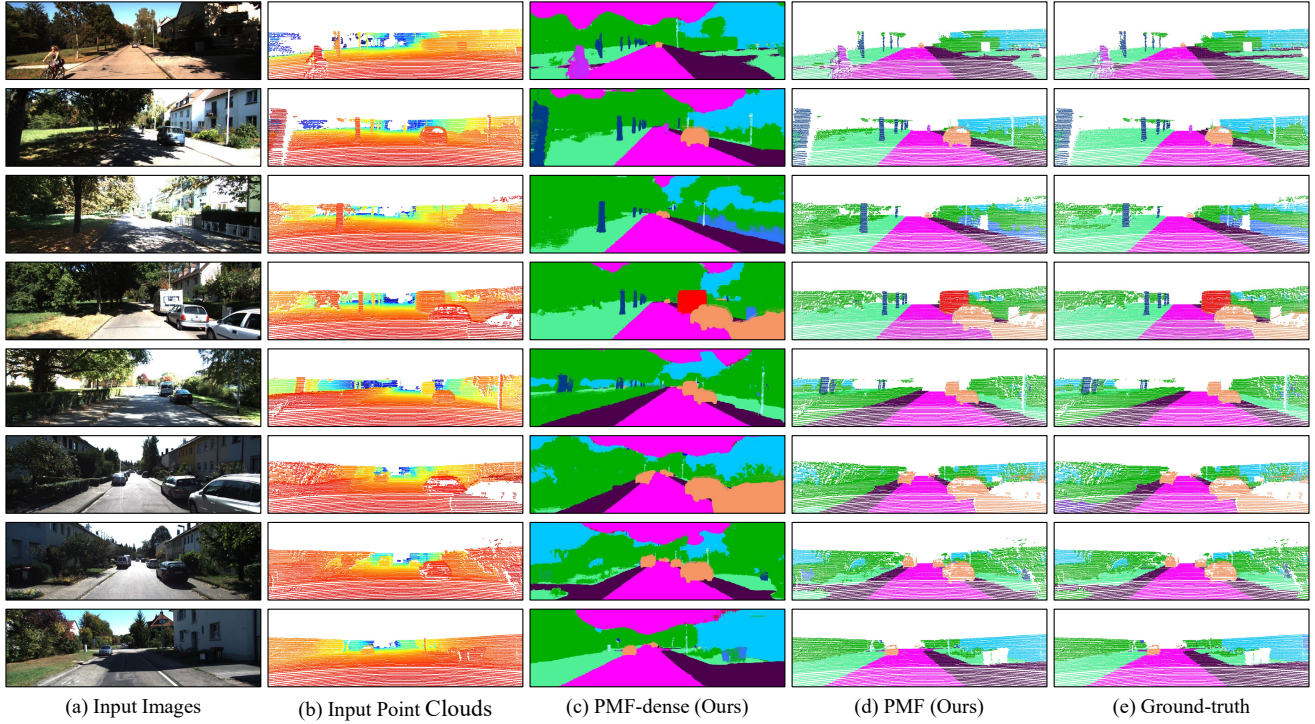

Figure V. More visualization results on SemanticKITTI. Better views by zoom in.

## 6. More Visualization Results on nuScenes

We provide more visualization results on nuScenes in Figure VI. From the results, our PMF shows its superiority on more challenging scenes, *i.e.*, night-time and sparse point clouds. For example, as shown in the 5-th to 8-th row in Figure VI, our PMF still performs well when most of the information from RGB images is missing at night. These results suggest that our method can address the segmentation with different lighting conditions.

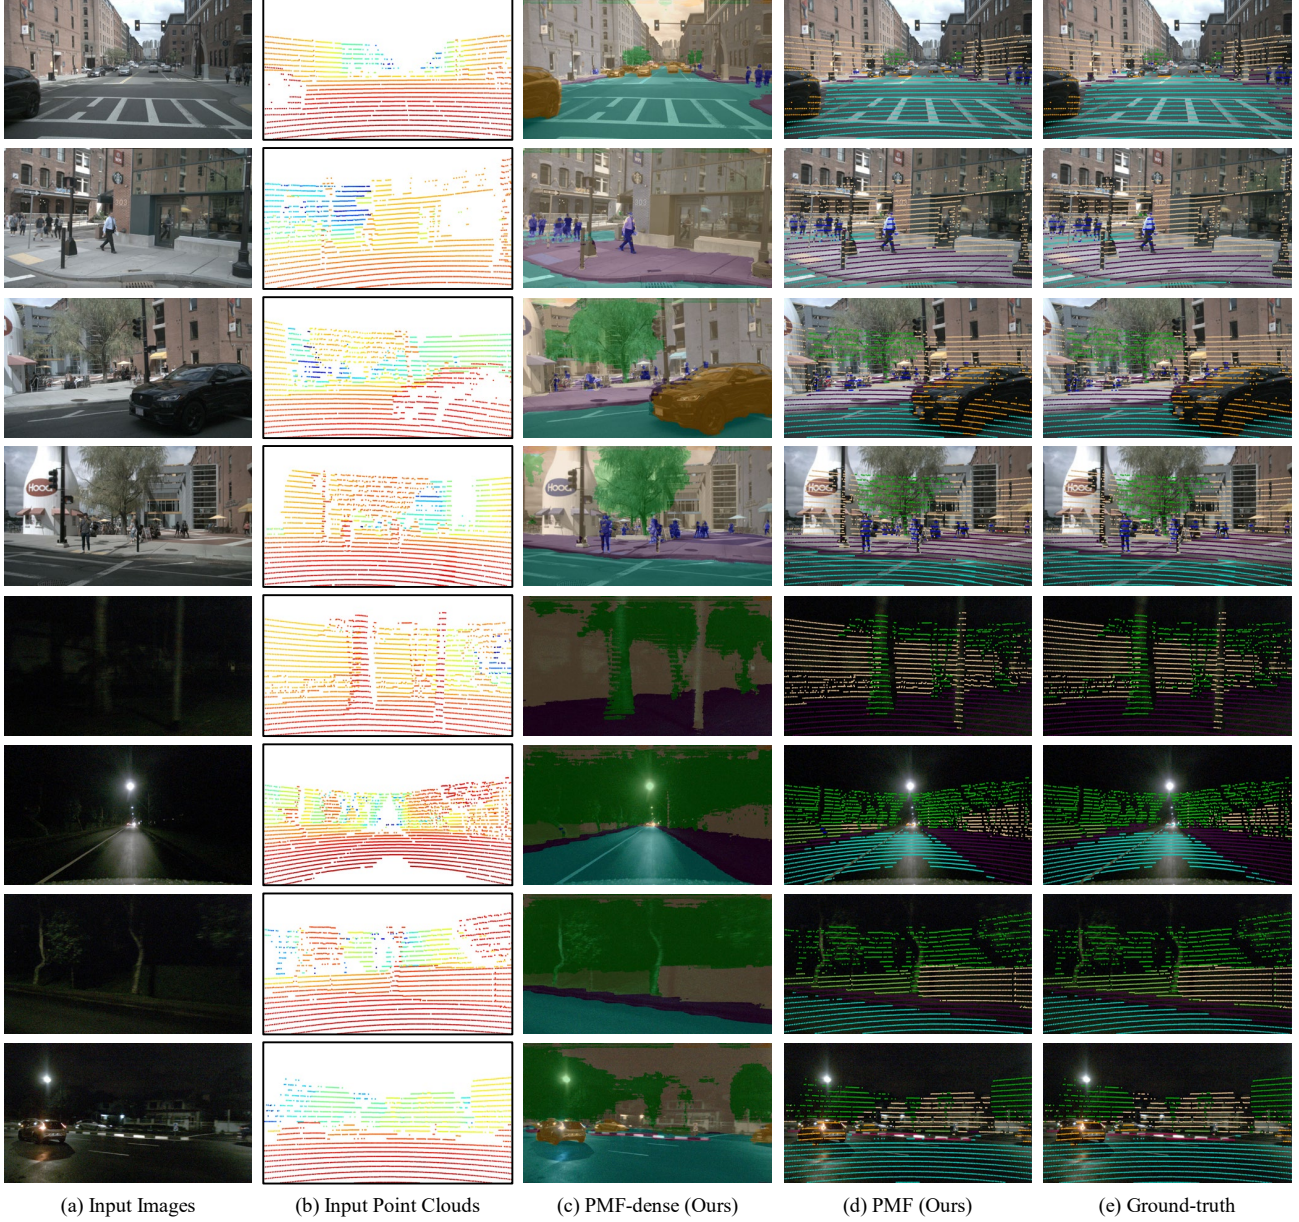

Figure VI. More visualization results on nuScenes. Better views by zoom in.

## 7. More Visualization Results on Adversarial Samples

We provide more results of PMF on adversarial samples in Figure VII. To obtain the adversarial samples, we insert extract objects, *i.e.*, car, traffic sign, bicyclist, into RGB images and keeping the point clouds no changed. From the results, our PMF reduces most of the noises from the images and is more robust to the adversarial samples than the camera-based methods.

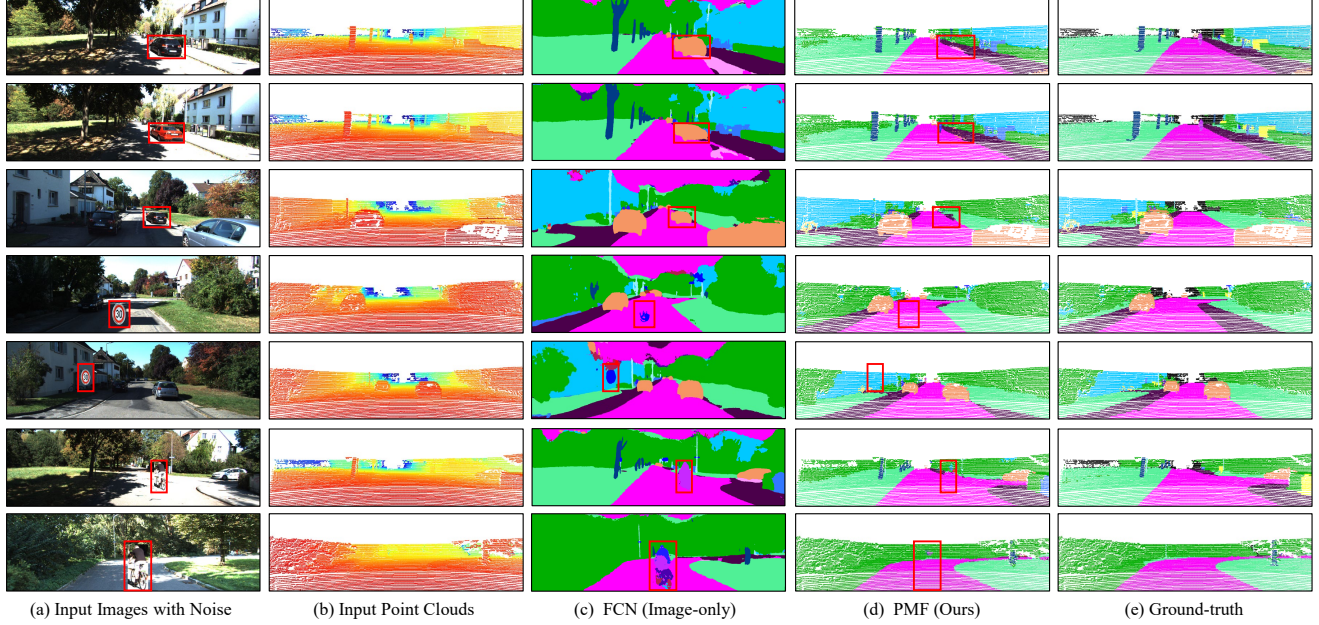

Figure VII. More visualization results of PMF on adversarial samples. FCN only uses RGB images as inputs, while PMF uses both RGB images and point clouds as inputs. We highlight the position of the inserted objects by red boxes. Better views by zoom in.

## References

- [1] Maxim Berman, Amal Rannen Triki, and Matthew B Blaschko. The lovász-softmax loss: A tractable surrogate for the optimization of the intersection-over-union measure in neural networks. In *IEEE Conference on Computer Vision and Pattern Recognition*, pages 4413–4421, 2018. 1
- [2] Tiago Cortinhal, George Tzelepis, and Eren Erdal Aksoy. Salsanext: Fast semantic segmentation of lidar point clouds for autonomous driving. *arXiv preprint arXiv:2003.03653*, 2020. 1
- [3] Georg Krispel, Michael Opitz, Georg Waltner, Horst Possegger, and Horst Bischof. Fuseseg: Lidar point cloud segmentation fusing multi-modal data. In *The IEEE Winter Conference on Applications of Computer Vision*, pages 1874–1883, 2020. 3
- [4] Tsung-Yi Lin, Priya Goyal, Ross Girshick, Kaiming He, and Piotr Dollár. Focal loss for dense object detection. In *IEEE International Conference on Computer Vision*, pages 2980–2988, 2017. 1
- [5] Khaled El Madawy, H. Rashed, Ahmad El Sallab, O. Nasr, H. Kamel, and S. Yogamani. Rgb and lidar fusion based 3d semantic segmentation for autonomous driving. *IEEE Intelligent Transportation Systems Conference*, pages 7–12, 2019. 3
- [6] Xinge Zhu, Hui Zhou, Tai Wang, Fangzhou Hong, Yuexin Ma, Wei Li, Hongsheng Li, and Dahua Lin. Cylindrical and asymmetrical 3d convolution networks for lidar segmentation. In *IEEE Conference on Computer Vision and Pattern Recognition*, pages 9939–9948, 2021. 1
